# Supplementary material for: Slow coarsening in jammed athermal soft particle suspensions
Source: arXiv:1903.00991 ancillary file (2019-08-08)
Supplement: Supplementary file 1 [file SM.pdf]

# Supplemental Material for
# "Slow coarsening in jammed athermal soft particle suspensions"


R. N. Chacko,[1] P. Sollich,[2] and S. M. Fielding[1]

[1] *Department of Physics, Durham University, Science Laboratories, South Road, Durham DH1 3LE, United Kingdom*

[2] *University of Göttingen, Institute for Theoretical Physics, 37077 Göttingen, Germany*



(Dated: July 17, 2019)


In the main text, we showed mostly the results of simulations performed in $d = 2$ spatial dimensions, for a sample prepared at time $t = 0$ by an instantaneous quench to zero temperature $T = 0$ from a previously infinite temperature, and for a sample size of $N = 10^6$ particles. In this Supplemental Material, we present corresponding results for simulations performed in $d = 3$ dimensions, for a sample prepared instead by a rapid particle swelling, and for sample sizes $N < 10^6$. As will be seen, our principal findings are robust against these changes, showing dimensionality, sample preparation, and system size to be unimportant to the basic physical picture.

*Effect of dimensionality* — In Fig. 1, we show the normalised spatial correlation functions of the thresholded (top 10%) particle speed maps for simulations performed in $d = 3$ dimensions. As seen for $d = 2$ in Fig. 4 of the main text, the associated correlation length $l^*$ increases as a power law of time $t$, although with an exponent that depends on the dimensionality: whereas in $d = 2$ we found $l^* \propto t^{0.36}$, in $d = 3$ we find $l^* \propto t^{0.24}$.

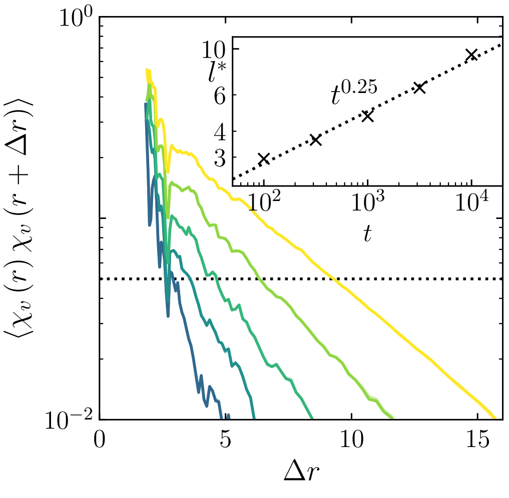


FIG. 1. Spatial correlation function of the thresholded particle speed $\chi_v$ for a three-dimensional system at volume fraction $\phi = 0.7$ at times $t = 10^2$, $10^3$ and $10^4$ in curves rightwards. Inset shows the dependence on time of the value $l^*$ of $\Delta r$ at which the correlator first falls below a threshold value 0.05, with the dotted line showing a fit to the power $t^{0.25}$.

In Fig. 2, we show snapshot colour maps of slices through the system at fixed $z$ for simulations in $d = 3$ spatial dimensions. These are counterpart to the colour maps shown in Fig. 2 of the main text for $d = 2$ dimensions. At any fixed time, localised hot-spots of high particle speed, rapidly changing particle energy, and high non-affine deformation rate are evident, as in $d = 2$. With increasing time in rows downwards, the patterns coarsen, with the hot-spots becoming progressively larger and further apart, also as in $d = 2$.

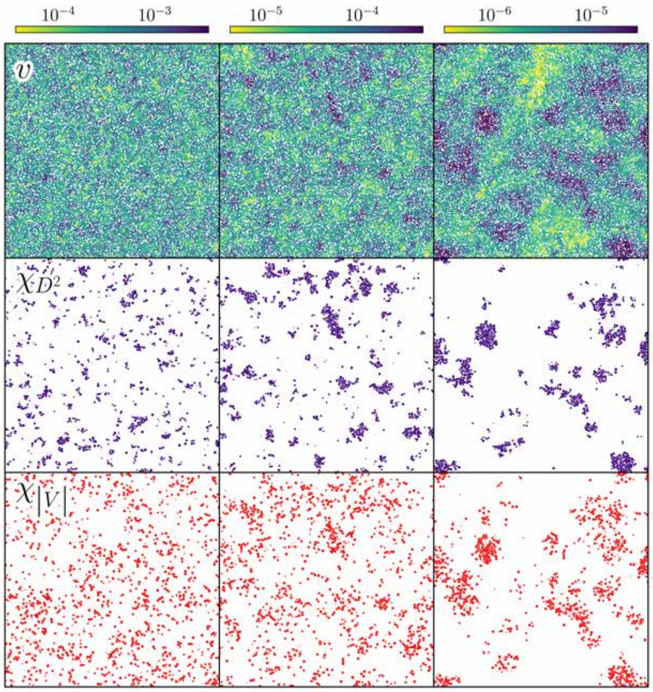


FIG. 2. Snapshot colourmaps for simulations in $d = 3$ dimensions of all particles that intersect the plane $z = L/2$. Columns rightwards show data at times $t = 10^3$, $10^4$ and $10^5$ for (top) particle speeds $v$, (centre) thresholded non-affine deformation rate $\chi_{D^2}$ and (bottom) thresholded magnitude of rate of change of particle energy $\chi_{|\dot{V}|}$. The colour scale for $v$ is centred around the most probable value $\log_{10} v$. Thresholded plots show particles in colour if they are within the top 10% as ranked by the quantity in question, and in white otherwise. Corresponding results for $d = 2$ are shown in Fig. 2 of the main text.

*Effect of initial sample preparation* — In the main text, we showed the results of simulations in which the particles are placed in the simulation box at time $t = 0$ with

uniformly distributed positions, corresponding to a sudden quench to temperature $T = 0$ from a previously infinite temperature. To demonstrate the robustness of our findings to changes in this initial condition, we now consider a different method of sample preparation, in which the assembly is initially equilibrated at a reduced volume fraction, $\phi = 0.5 < \phi_{\rm J}$, and nonzero temperature $T = 0.01$, before suddenly expanding the particles in situ at time $t = 0$ to achieve the desired $\phi > \phi_{\rm J}$, and setting $T = 0$. This is intended to model the rapid swelling of core-shell particles to reach a jammed state. As shown in Fig. 3, we find the same dynamical scenario for both of these initial conditions, including a non-trivial power-law decay of the root mean squared particle speed, with power laws that coincide beyond an initial transient.

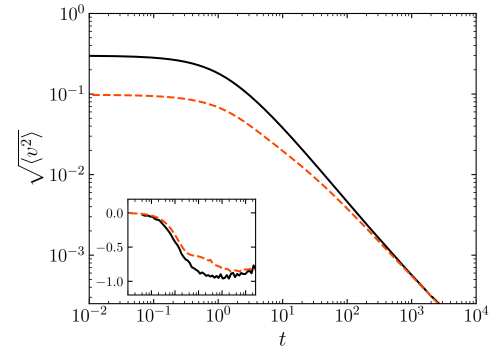


FIG. 3. Decay of the root mean squared particle speed for (black solid line) a three-dimensional system quenched at time $t = 0$ from temperature $T = \infty$ to $T = 0$ compared with that (red dashed line) for a system equilibrated at $\phi = 0.5$ and $T = 0.01$ before at $t = 0$ being quenched to $T = 0$ and compressed to $\phi = 0.7$. Inset shows $\partial \ln(\sqrt{\langle v^2\rangle})/\partial \ln t$.

*Effect of finite system size* — In the main text, we displayed the results of simulations performed with $N = 10^6$ particles. In Fig. 4, we show the outcome of simulations for several different values of the system size. As can be seen, for any fixed $N$ the power law decay of the root mean squared particle speed eventually terminates in noise. The time at which this occurs increases with increasing $N$, such that in the limit $N \to \infty$ we anticipate the power law would persist indefinitely.

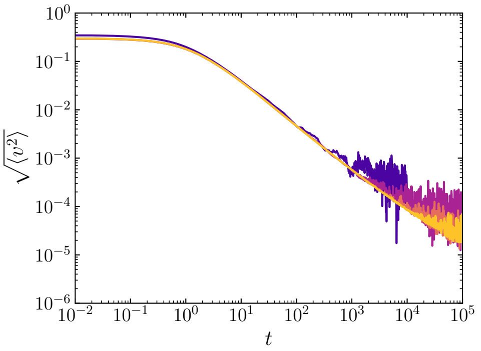


FIG. 4. Decay of the root mean squared particle speed for system sizes of $N = 10^3$, $10^4$, $10^5$ and $10^6$ particles. Lighter curves correspond to larger $N$. The time at which the power law decay gives way to noise increases with increasing $N$. Dimensionality $d = 3$, volume fraction $\phi = 0.7$.

*Thresholding choices* — In Fig. 4a of the main text and Fig. 1 of this Supplemental Material, we show data for the spatial correlation function of the thresholded speed $\chi_v$, defined such that $\chi_v = 1$ at a particle's position if that particle's speed is within the top 10% of all particle speeds, with $\chi_v = 0$ otherwise. In Fig. 5, we show the spatial correlation function for a more selective choice of threshold, $\chi_v^{1\%}$, defined such that $\chi_v^{1\%} = 1$ at particles within the top 1% as ranked by speed, $\chi_v^{1\%} = 0$ otherwise. We see that we still obtain a power law, with a somewhat smaller exponent.

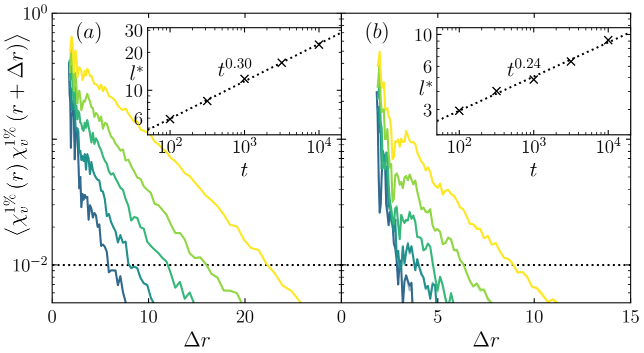


FIG. 5. Normalised spatial correlation function of the thresholded particle speed $\chi_v^{1\%}$ at times $t = 10^2$, $10^3$ and $10^4$ in curves rightwards for $(a)$ a two-dimensional system at volume fraction $\phi = 0.9$ and $(b)$ a three-dimensional system at volume fraction $\phi = 0.7$. Inset shows the dependence on time of the value $l^*$ of $\Delta r$ at which the correlator first falls below a threshold value 0.01, with the dotted line showing a fit to a power law.

We also show, in Fig. 6, the correlation function obtained with a different style of thresholding. Here, a particle has thresholded speed $K_v = 1$ if its speed is more than three times the mean particle speed, $K_v = 0$ otherwise. This time, we obtain power laws with a larger

exponent than when using $\chi_v$.

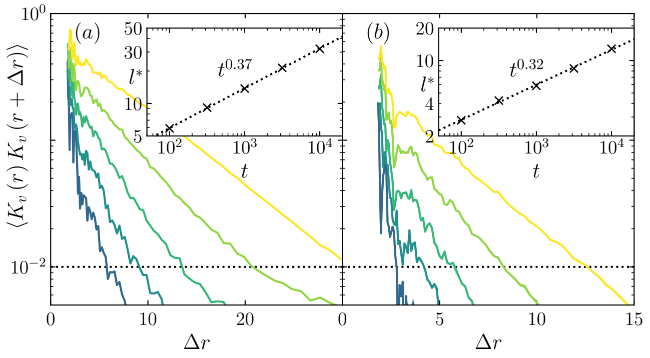


FIG. 6. Normalised spatial correlation function of the thresholded particle speed $K_v$ at times $t = 10^2$, $10^3$ and $10^4$ in curves rightwards for $(a)$ a two-dimensional system at volume fraction $\phi = 0.9$ and $(b)$ a three-dimensional system at volume fraction $\phi = 0.7$. Inset shows the dependence on time of the value $l^*$ of $\Delta r$ at which the correlator first falls below a threshold value 0.01, with the dotted line showing a fit to a power law.

Finally, in Fig. 7, we show the normalised correlation function of the particle speed $v$ without any thresholding. We identify power law exponents 0.42 in two dimensions, and 0.32 in three dimensions.

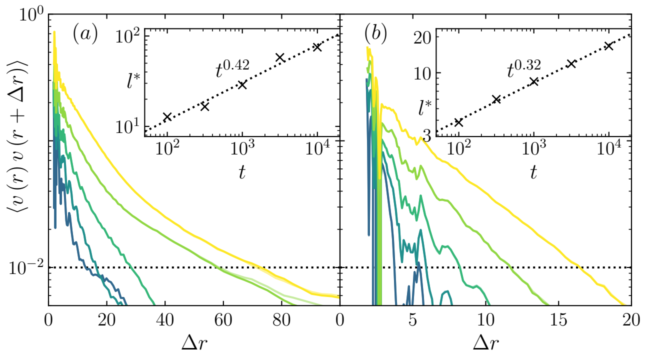


FIG. 7. Normalised spatial correlation function of the particle speed $v$ at times $t = 10^2$, $10^3$ and $10^4$ in curves rightwards for $(a)$ a two-dimensional system at volume fraction $\phi = 0.9$ and $(b)$ a three-dimensional system at volume fraction $\phi = 0.7$. Inset shows the dependence on time of the value $l^*$ of $\Delta r$ at which the correlator first falls below a threshold value 0.01, with the dotted line showing a fit to a power law.

We note that the exponents are insensitive to the correlator value chosen in the definition of $l^*$, so long as the value is small enough that all the correlator curves are in their long-$\Delta r$ descent, but large enough that the noise of the decorrelated portion of the curve is avoided.

From the variation in the exponents above (0.37, 0.30, 0.37, 0.42 in $d = 2$, 0.25, 0.24, 0.32, 0.32 in $d = 3$), we estimate a growth exponent of 0.37 in $d = 2$ and 0.28 in $d = 3$, with an uncertainty of $\pm 0.04$ in both cases.

*Supplemental Movie* — We include a movie `movie.avi` showing the evolution of $\dot{V}/|<\dot{V}>|$ in the region shown in Fig. 3 of the main text across a period of time straddling the events shown there.
